# Supplementary material for: Enhanced molecular spin-photon coupling at superconducting nanoconstrictions
Source: arXiv:2006.03386 ancillary file (2020-06-05)
Supplement: Supplementary file 1 [file acs-Gimeno_ACSnano_SI.pdf]

# Template for Submission of Manuscripts to American Chemical Society Journals

### Word 2010, single-column, double-spaced (2013)

This template is a guide to be used to prepare manuscripts for submission. Please consult the Instructions to Authors or a recent issue of the journal for detailed guidelines and procedures for submission. This template is intended to benefit to the author in that the entire manuscript (text, tables, and graphics) may be submitted in one file. Inserting graphics and tables close to the point at which they are discussed in the text of the manuscript can also be a benefit for the reviewer.

When you submit a manuscript using this template, you will not actually see the page formatting that appears in the printed journal. This will occur as part of the editorial production process. Abbreviated instructions for using the template follow. Consult the documentation for your specific application and version for more information. Additional instructions can be found in the readme file at the web page where you downloaded this template.

**Using the template**

In ACS publications there are many different components of a manuscript (i.e., title, abstract, main text, figure captions, etc.) that are represented in the template. See the Guide, Notes, Notice, or Instructions for Authors on the journal's homepage to determine which parts should be included for the manuscript that you are preparing

1. If typing your manuscript directly into the template, select (highlight) the text of the template that you want to replace and begin typing your manuscript (i.e., select the Title section for typing in your title).
2. If you have already prepared your document in a Word file, you will need to attach the template to your working document in order to apply the Word Style tags. Further instructions can be found in the readme file at the web page where you downloaded this template.
    a. Go to the Add-Ins tab and you will see all the Word Styles from the template that has now been imported into the current document. A Styles toolbar has been generated that will display the different Styles for you to choose from. If this is not present, type in the following command (Alt+Ctrl+Shift+S) and it should appear. You can close this at any time and then reopen it when needed.
    b. Click in the sentence or paragraph and then go to the Add-Ins tab and select the relevant Word Style. This will apply the Word Style to the entire text (sentence or paragraph). Do this for all sections of the manuscript.
3. To insert graphics within the text or as a figure, chart, scheme, or table, create a new line and insert the graphic where desired. If your graphic is not visible, ensure that the Word Style is "Normal" with an automatic height adjustment. If the size of the artwork needs to be adjusted, re-size the artwork in your graphics program and re-paste the artwork into the template (maximum width for single-column artwork, 3.3 in. (8.5 cm); maximum width for double-column artwork, 7 in. (17.8 cm)). **NOTE**: If you are submitting a Table of Contents graphic, please insert the graphic at the end of the file.
4. Ensure that page numbers are present on all pages before submitting your manuscript.
5. Delete these instructions and any sections that are not needed.
6. Save the file with the graphics in place: select **Save As** (**File** menu) and save it as a document file (not a .dot template file).
7. Proof the manuscript to ensure that all parts of the manuscript are present and clearly legible.

# Supplementary information for “Enhanced molecular spin-photon coupling at superconducting nanoconstrictions”

*Ignacio Gimeno,[1] Wenzel Kersten,[2] María C. Pallarés,[3] Pablo Hermosilla,[3] María José Martínez-Pérez, [1,4] Mark Jenkins,[1] Andreas Angerer,[2] Carlos Sánchez-Azqueta,[5] David Zueco,[1,4] Johannes Majer,[2,6,7] Anabel Lostao,[1,3,4] and Fernando Luis[1,*]*

[1]Instituto de Ciencia de Materiales de Aragón, CSIC-Universidad de Zaragoza, Pedro Cerbuna 12, 50009 Zaragoza, Spain

[2]Vienna Center for Quantum Science and Technology, Atominstitut, TU Wien, 1020 Vienna, Austria.

[3]Laboratorio de Microscopías Avanzadas, Instituto de Nanociencia de Aragón, Universidad de Zaragoza, 50018 Zaragoza, Spain

[4]Fundación ARAID, Campus Río Ebro, 50018 Zaragoza, Spain

[5]Departamento de Física Aplicada, Universidad de Zaragoza, 50009 Zaragoza, Spain.

[6]Shanghai Branch, CAS Center for Excellence and Synergetic Innovation Center in Quantum Information and Quantum Physics, University of Science and Technology of China, Shanghai 201315, China

[7]National Laboratory for Physical Sciences at Microscale and Department of Modern Physics, University of Science and Technology of China, Hefei 230026, China

**Corresponding Author**

*fluis@unizar.es

1. FABRICATION OF SUPERCONDUCTING RESONATORS WITH NANOSCOPIC CONSTRICTIONS

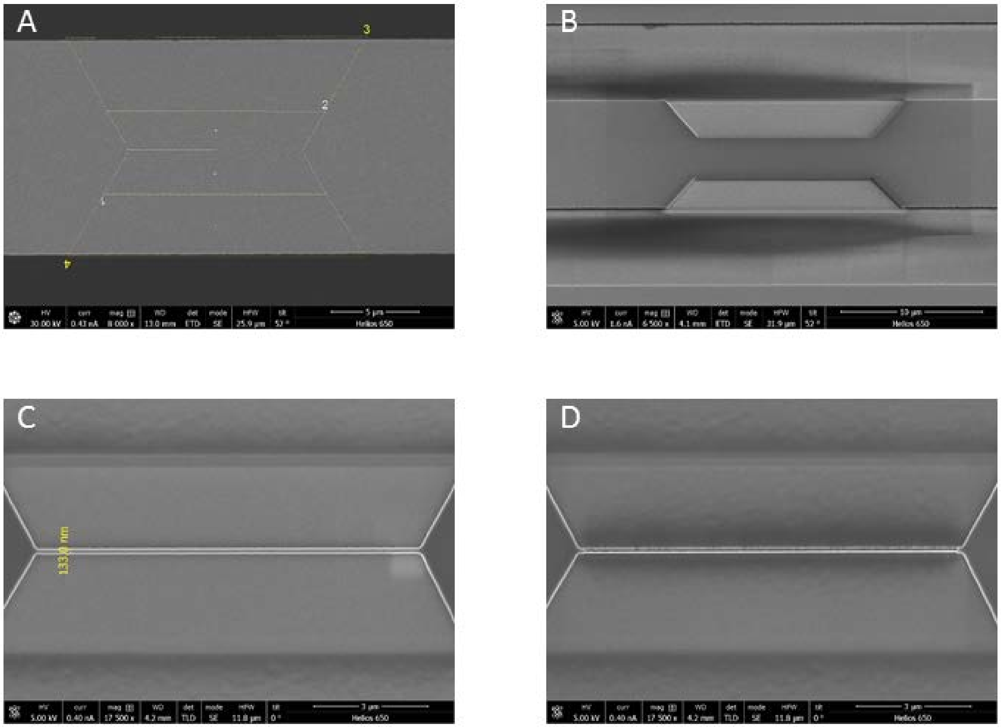


**Figure S1. Fabrication steps of a superconducting nanoconstriction** at the center of the transmission line of a coplanar superconducting resonator. A $Ga^{+}$ ion beam is focused onto the central line to progressively thin it down to about 42 nm.

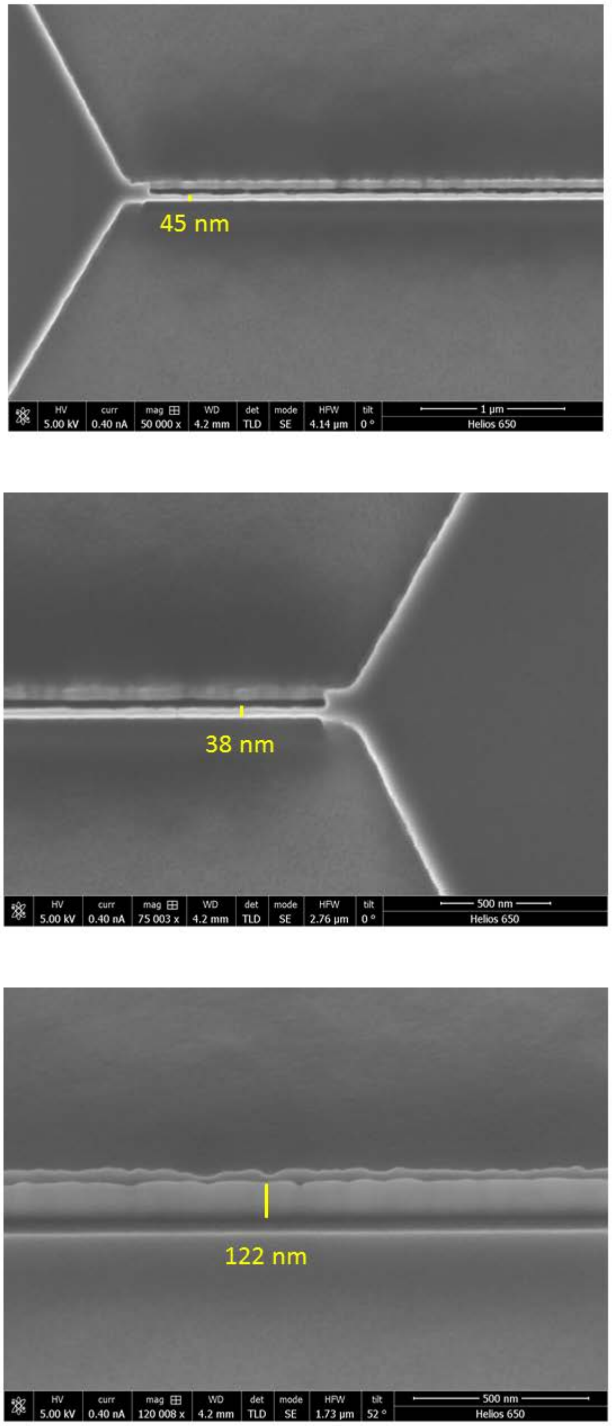


**Figure S2. Close-up SEM images** of the resulting 38-45 nm wide, 122 nm high constriction.

2. CHARACTERIZATION OF SUPERCONDUCTING RESONATORS WITH NANOSCOPIC CONSTRICTIONS

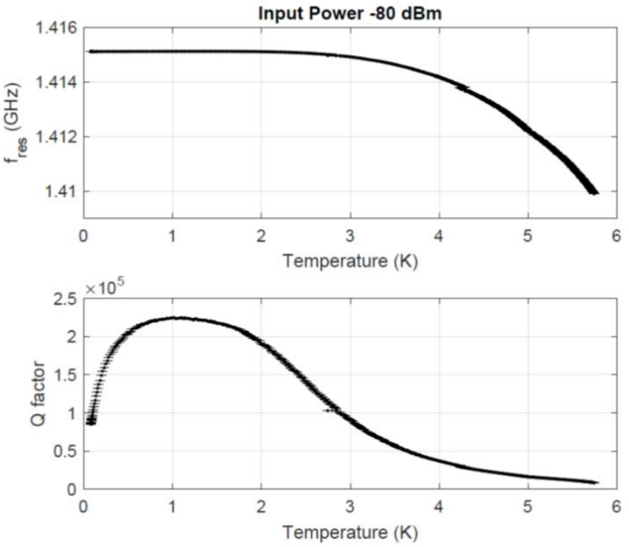


**Figure S3. Variation of the resonator characteristics with temperature.** Temperature dependence of the resonance frequency (top) and quality factor (bottom) of the resonator shown in figures S1 and S2.

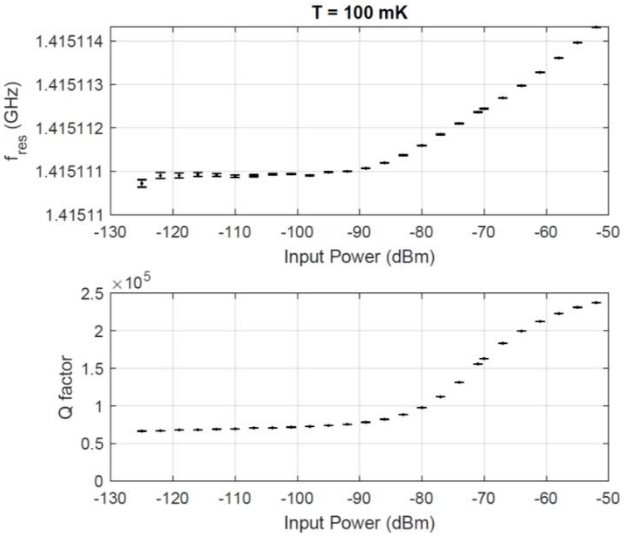

**Figure S4. Input power dependence** of the resonance frequency (top) and quality factor (bottom) of the resonator shown in figures S1 and S2 measured at a temperature of 100 mK.

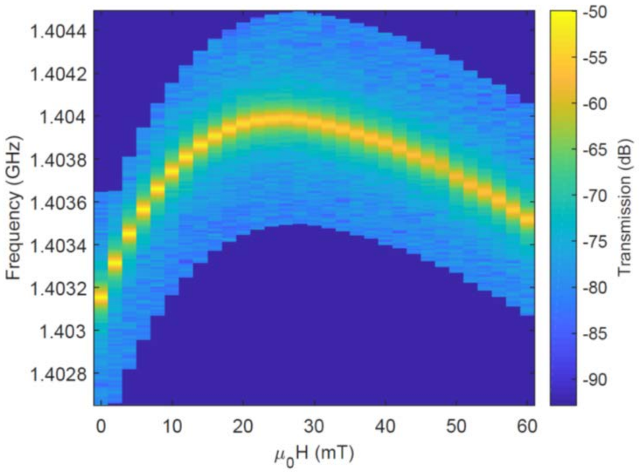


**Figure S5. Magnetic field dependence** of the resonant transmission of the resonator shown in Figs S1 and S2, measured at T = 45 mK.

3. MICROWAVE TRANSMISSION EXPERIMENTS: $w$ = 400 μm RESONATOR COUPLED TO A LARGE DPPH PELLET

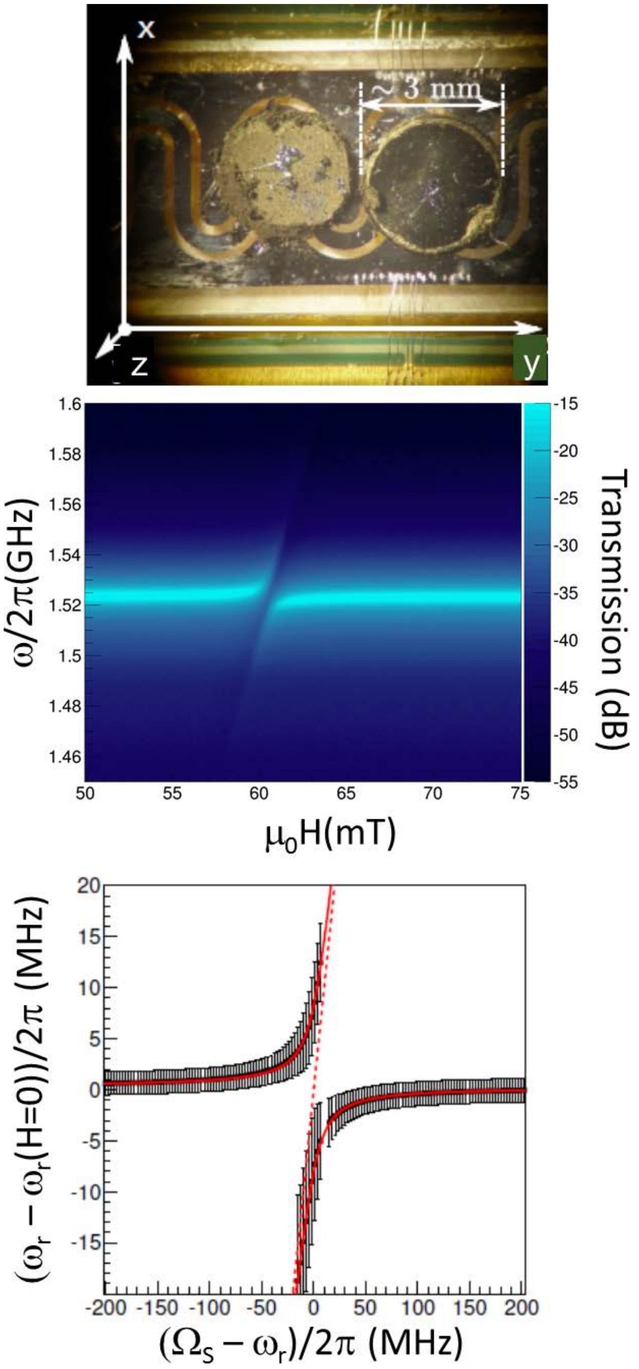


**Figure S6. Strong coupling of a large DPPH ensemble to a superconducting coplanar resonator.** Top: optical microscopy image of a superconducting coplanar resonator with a 400 μm

wide central transmission line hosting two pressed pellets of polycrystalline DPPH. Middle: 2D plot of the microwave transmission of this device measured at T = 4.2 K. Bottom: magnetic field dependence of the resonance frequency, showing the anti-crossing that is characteristic of the strong coupling regime. The solid lines are least-square fits to the equation $\omega_{\pm} = \frac{\omega_r+\Omega_S}{2} \pm \frac{\sqrt{4G_N^2+(\Omega_S-\omega_r)^2}}{2}$, which is valid in this coupling limit and that allows determining $G_N$ = 8.2 MHz.

4. DEPOSITION OF DPPH ORGANIC RADICALS BY DIP-PEN NANOLITHOGRAPHY

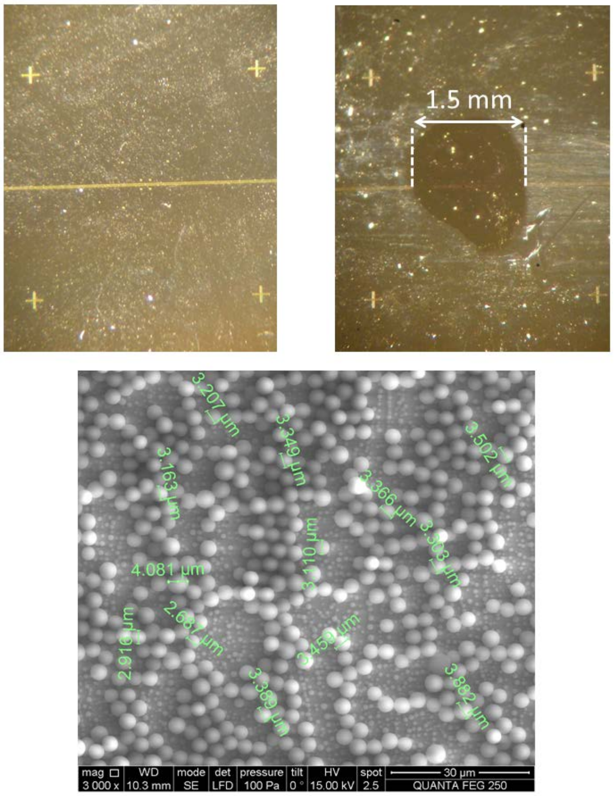


**Figure S7. Deposition of macroscopic DPPH ensembles.** Top: Optical microscopy images of a coplanar resonator (no constriction) before and after the deposition of a macroscopic drop of DPPH molecules. The deposition is done over the central region of the device, using a conventional

micropipette. Bottom: SEM image of the deposit after the solvent has evaporated, showing the tendency of DPPH to form aggregates.

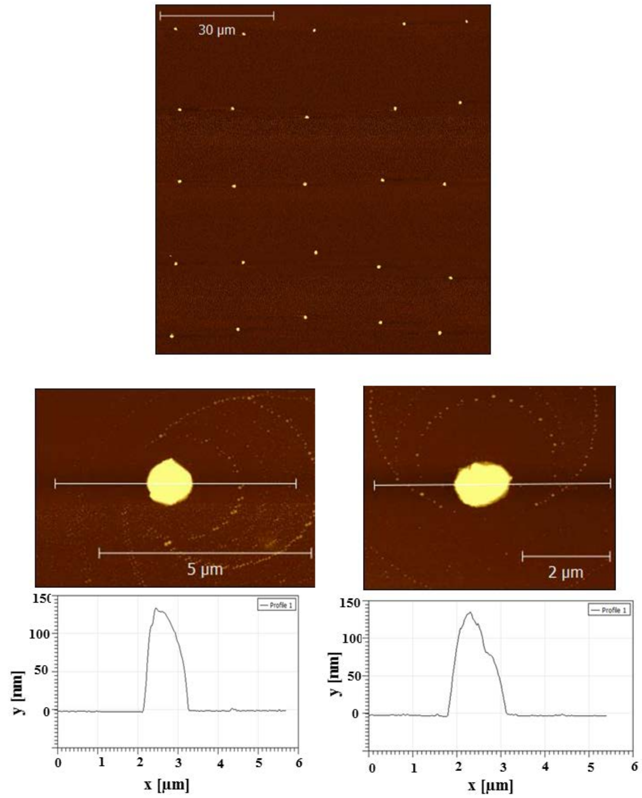


**Figure S8. Control over the size and location of DPPH deposits by dip-pen nanolithography (DPN).** Top: AFM image of an array of DPPH nanodroplets deposited onto a mica substrate by dip-pen nanolithography. Bottom: AFM topography images and height profiles of two of the dots measured after the solvent had evaporated.

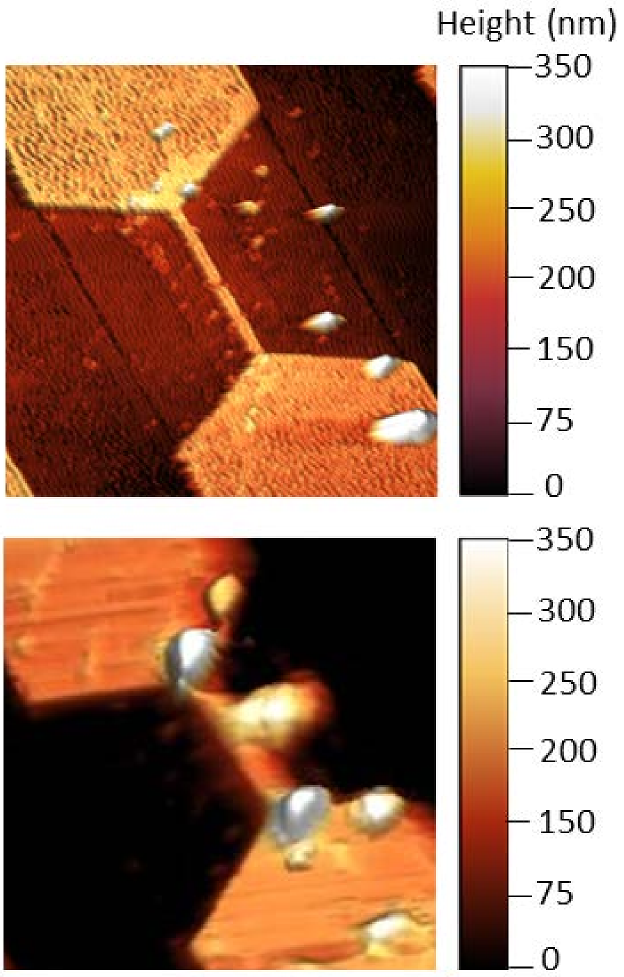


**Figure S9. Deposition of DPPH nanodroplets onto superconducting nanoconstrictions.** AFM 3D topography images of the same 158 nm wide constriction after two different depositions of DPPH by DPN. The one at the top gives a coupling to the resonator that is barely above the sensitivity of the experimental set-up, as no molecular nano-agglomerate has "landed" next to the constriction.

5. DETERMINATION OF THE NUMBER N OF MOLECULAR SPINS WITHIN THE "ACTIVE" REGION OF A NANOCONSTRICTION

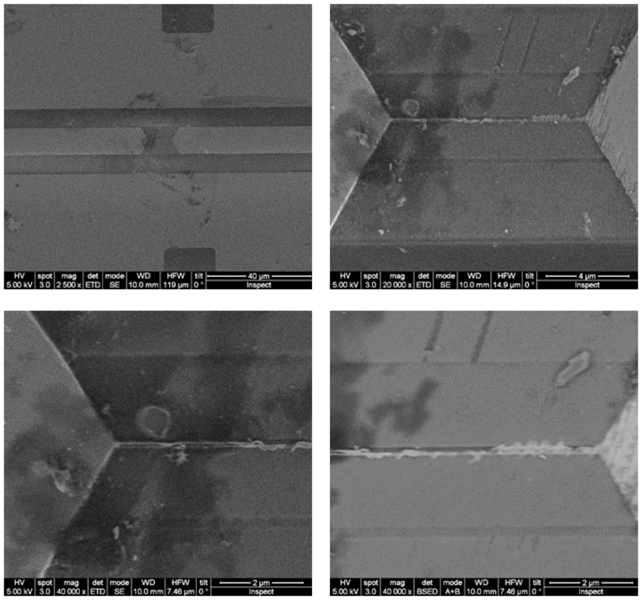

**Figure S10. Characterization of DPPH deposits by Scanning Electron Microscopy (SEM).** SEM images of the central region of a resonator with a 38-45 nm wide constriction. Dark areas correspond to remains of glycerol, whereas bright spots correspond to DPPH nano-agglomerates.

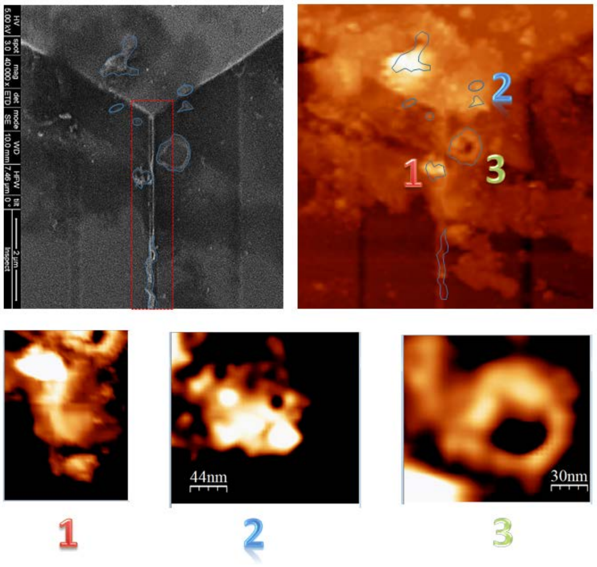


**Figure S11. Determination of the number of DPPH molecules deposited.** Top: SEM (left) and AFM (right) images of the same region near the nano-constriction. Bright contrast in the SEM images signals the presence of DPPH molecules (see also Figs. S7 and S10). AFM topographic images are used to estimate the volume of all DPPH nano-agglomerates that are within 500 nm distance from the constriction (red dotted rectangle). The bottom figures show AFM images of three of these agglomerates.

6. CALCULATION OF THE COLLECTIVE COUPLING TO THE RESONATOR

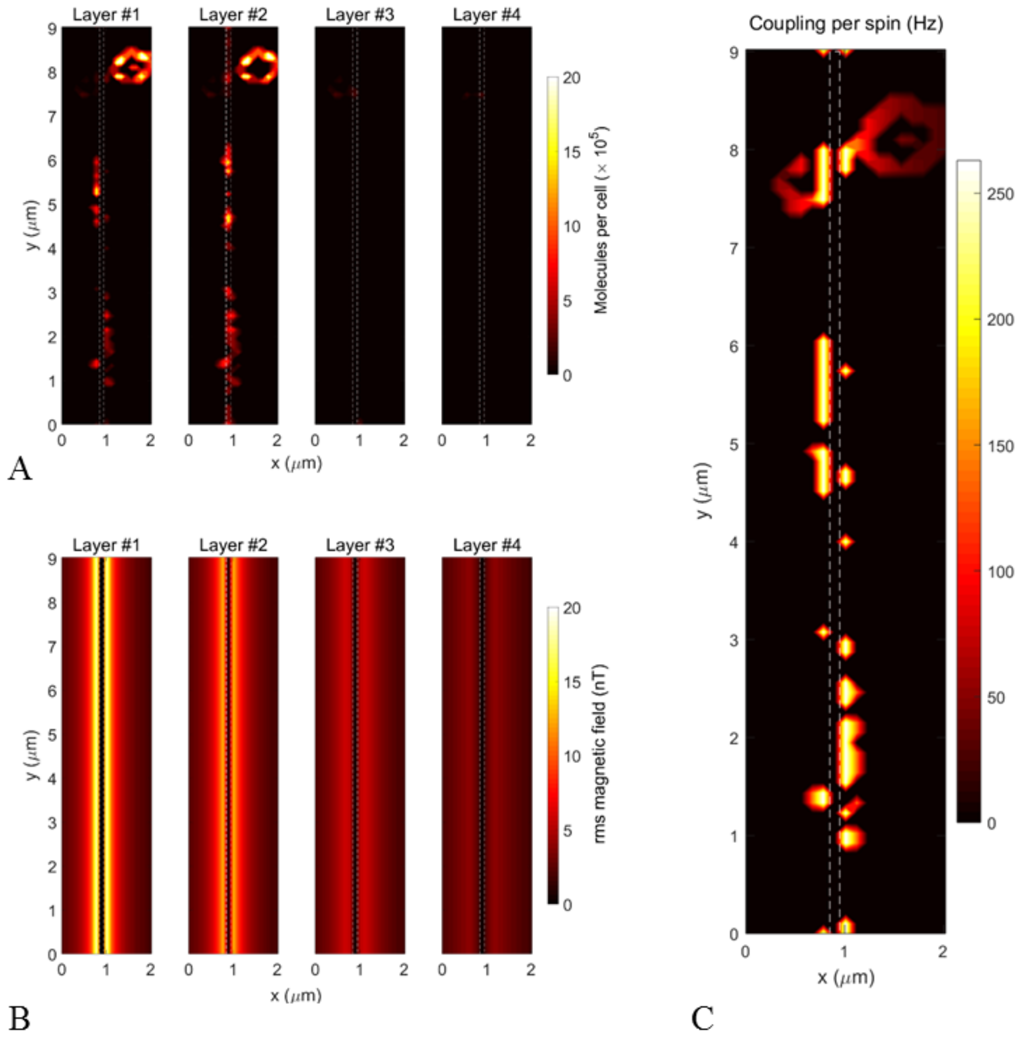


**Figure S12. Finite elements calculation of the spin-photon coupling (magnetic field parallel to x).** A: distribution of DPPH molecules in a three-dimensional grid centered over a 42 nm wide constriction. The cell size was 100×100×100 nm$^3$. The image shows the distributions in four layers located progressively farther from the chip surface (from left to right, starting from the one lying on the chip’s surface). B: z component of the magnetic field b generated by a photon at the center

of each cell. This is the component that contributes to the spin-photon coupling when the external magnetic field points along the x axis, as in the experiments described in Fig. 5 of the main text. Notice that this component vanishes at the top of the central line as indicated by the black contrast. C: Resulting maximum coupling energy per spin. The coupling is reduced just above the nano-constriction as a result of the vanishing $b_z$.

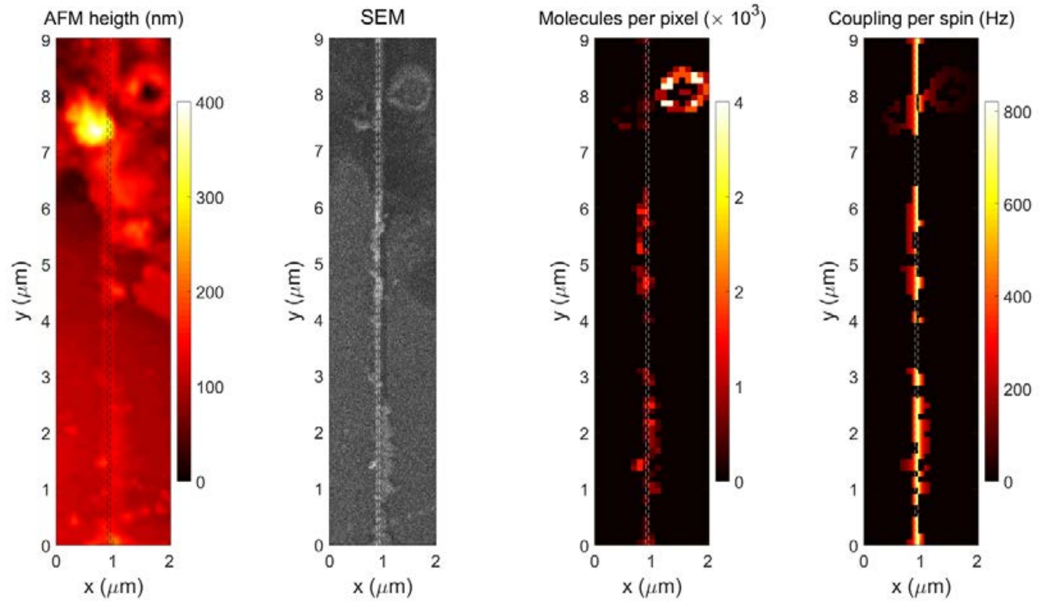


**Figure S13. Spin-photon coupling for the optimal field orientation (magnetic field along y).** From left to right: AFM and SEM images of the region near a 42 nm wide nano-constriction, color map of the number of DPPH molecules deposited on each location, and color map of the estimated single spin to photon couplings. The latter maps have been calculated with a discretization of space into 3×3×3 $nm^3$ cubic cells and for a magnetic field applied along the z axis, which maximizes the coupling. The number of free-radical molecules deposited in this area amounts to approximately $N = 1.6\times10^8$ and the collective coupling estimated from the simulations is $G_N / 2\pi = 2.6$ MHz at T

= 44 mK and 3.3 MHz at T = 0. The maximum coupling reaches values above 0.8 kHz for spins located in the close proximity of the central line.

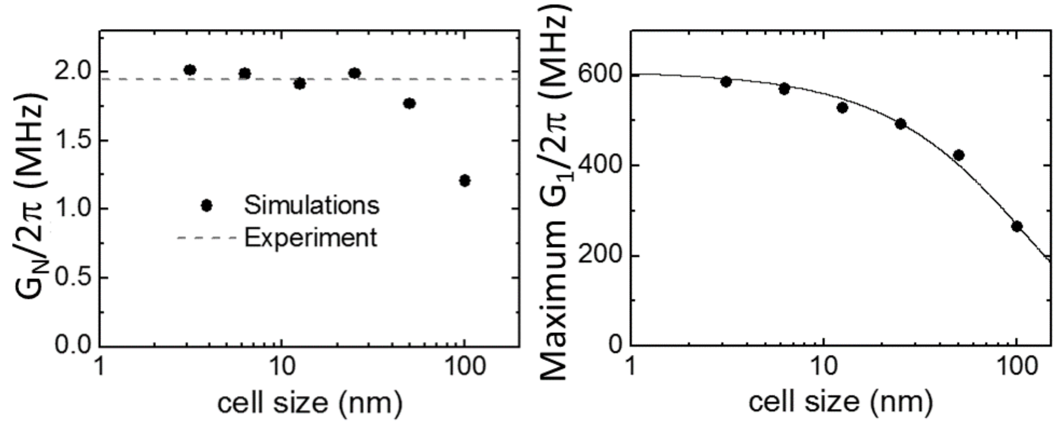


**Figure S14. Determination of the optimum cell size.** Collective spin-photon coupling (left) and maximum single-spin coupling energies calculated for the situation shown in Fig. S12 for varying size of the cells that form the grid. The calculations of $G_N$ were performed for T = 44 mK, which corresponds to the experimental conditions of the results shown in Fig. 5 of the main text.

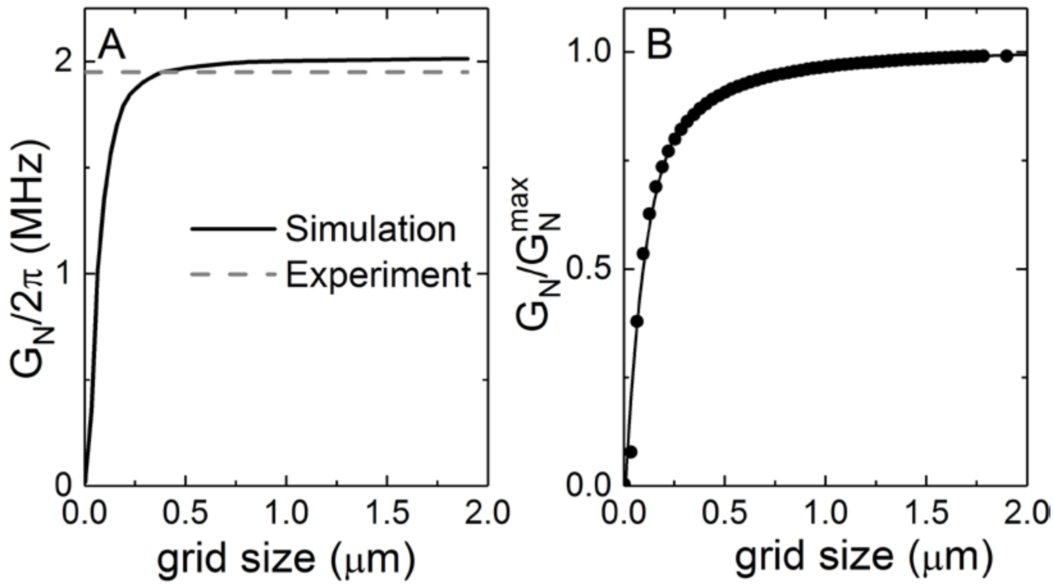


**Figure S15. Determination of the optimum grid size: effective mode volume of a resonator near a superconducting nano-constriction.** A: Collective spin-photon coupling calculated for the situation shown in Fig. S12 for varying size of the grid and a fixed cell size d = 3 nm. The calculations were performed for T = 44 mK, which corresponds to the experimental conditions of the results shown in Fig. 5 of the main text. The results show that spins located beyond a distance of about 500 nm from the constriction give a close to negligible contribution. B: Results of the same calculation for the case of a homogeneously distributed molecular deposit. The width of the region that contributes most to the coupling becomes then about two times larger, showing that the coupling enhancement in A results from two combined effects: the reduce central line width and the ability to locate molecules in the optimum positions with respect to the constriction. From these results, the effective mode volume can be estimated as ≈ 1 μm × 1 μm × 10 μm = 10 $\mu m^3$.

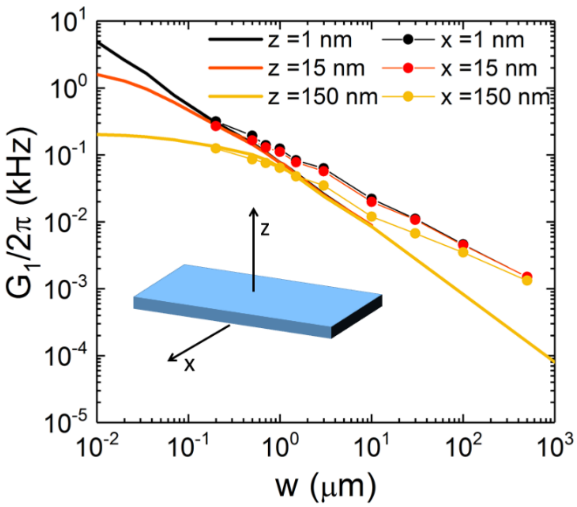


**Figure S16. Single-spin coupling versus constriction diameter.** Coupling to 1.4 GHz photons of individual spins located at a certain distance from the central line. As a result of the central line geometry (a slab having width w and a close to constant thickness t of about 120 nm for w > t and close to w otherwise), the coupling depends on whether the spins are over the central line, and then moved along the vertical z axis from the surface, or whether they are moved within the plane (along x). For w > 1 μm, the probability of finding spins near the line edges, which generate stronger magnetic fields, becomes very small. For w < 1 μm, the difference between both situations understandably vanishes. Therefore, the coupling to spins located over the central line provides a good estimation of the “typical” single spin coupling. This choice has been used in Fig. 6 of the main text.
